# Supplementary material for: Shirakami: A Hybrid Concurrency Control Protocol for Tsurugi Relational Database System
Source: arXiv:2303.18142 source file (2026-07-02)
Supplement: Supplementary file 1 [file appendix-alg.tex]

\section{Full Algorithm}

\begin{algorithm}[H]
\caption{Long Transaction Execution (LTX)}
\label{alg:ltx}
\DontPrintSemicolon
\FExecLTX{$tx$}\;
\Begin{
    $tx\_id \gets \text{assign\_transaction\_id}()$\;
    $commit\_epoch \gets \text{get\_global\_epoch}() + 1$\;
    $\text{register\_write\_preserves}(tx.wp\_storages, tx\_id, commit\_epoch)$ \tcp*{Storage-level}
    
    \tcp{Execution Phase}
    $overtaken\_set \gets \emptyset, read\_range \gets \emptyset, max\_read\_epoch \gets 0$\;
    
    \ForEach{$operation \in tx$}{
        \If{$operation.type \in \{\text{READ, SCAN}\}$}{
            $key\_or\_range \gets operation.key\_or\_range$\;
            \tcp{Detect higher priority LTX write-preserves}
            \ForEach{$\langle wp\_tx\_id, wp\_epoch \rangle \in \text{get\_write\_preserves}(\text{storage\_of}(key\_or\_range))$}{
                \If{$wp\_tx\_id < tx\_id$}{
                    $overtaken\_set \gets overtaken\_set \cup \{wp\_tx\_id\}$\;
                    $read\_range \gets read\_range \cup \{key\_or\_range\}$\;
                }
            }
            \tcp{Read snapshot}
            \eIf{$operation.type = \text{READ}$}{
                $value, version \gets \text{read\_snapshot}(operation.key, commit\_epoch)$\;
                $read\_set \gets read\_set \cup \{operation.key\}$\;
                $read\_epoch \gets version.epoch$\;
            }{
                $values, versions \gets \text{scan\_snapshot}(operation.range, commit\_epoch)$\;
                $range\_read\_set \gets range\_read\_set \cup \{operation.range\}$\;
                $read\_epoch \gets \text{max\_epoch\_from\_versions}(versions)$\;
            }
            $max\_read\_epoch \gets \max(max\_read\_epoch, read\_epoch)$\;
        }
        \Else{
            $write\_set \gets write\_set \cup \{operation\}$\;
        }
    }
    
    \tcp{Order Forwarding}
    \ForEach{$ltx\_id \in overtaken\_set$}{
        $\text{wait\_for\_completion}(ltx\_id)$\;
        \If{$\text{committed}(ltx\_id)$}{
            $ltx\_write\_range \gets \text{get\_write\_range}(ltx\_id)$\;
            \If{$\text{range\_overlap}(read\_range, ltx\_write\_range)$}{
                $ltx\_commit\_epoch \gets \text{get\_commit\_epoch}(ltx\_id)$\;
                $new\_epoch \gets \min(commit\_epoch, ltx\_commit\_epoch)$\;
                \If{$max\_read\_epoch \ge new\_epoch$}{
                    \Return{ABORT} \tcp*{Read upper bound violation}
                }
                $commit\_epoch \gets new\_epoch$\;
            }
        }
    }
    
    \tcp{Final Validation}
    \If{$\neg \FValidatePhantom{write\_set, commit\_epoch}$}{ \Return{ABORT} }
    \ForEach{$operation \in write\_set$}{
        \If{$commit\_epoch \le \text{get\_max\_reader\_epoch}(operation.key)$}{ \Return{ABORT} }
    }
    
    $\text{register\_reader\_epoch}(read\_set \cup range\_read\_set, commit\_epoch)$\;
    $\text{apply\_writes}(write\_set, commit\_epoch)$\;
    $\text{put\_write\_range}(tx\_id, write\_set)$\;
    $\text{cleanup\_write\_preserves}()$\;
    \Return{COMMIT}\;
}
\end{algorithm}

\begin{algorithm}[H]
\caption{OCC and RTX Execution}
\label{alg:occ_rtx}
\DontPrintSemicolon

\SetKwBlock{FnOCC}{function \FExecOCC{$tx$}}{end}
\FnOCC{
    \ForEach{$op \in tx$}{
        \eIf{$op.type \in \{\text{READ, SCAN}\}$}{
            \eIf{$op.type = \text{READ}$}{
                $v, ver \gets \text{read\_latest}(op.key)$\;
                $read\_set \gets read\_set \cup \{\langle op.key, ver \rangle\}$\;
                $read\_storages \gets read\_storages \cup \{op.storage\}$\;
            }{
                $node\_set \gets node\_set \cup \{\text{accessed\_nodes}\}$\;
                $scan\_storages \gets scan\_storages \cup \{op.storage\}$\;
            }
        }{
            $write\_set \gets write\_set \cup \{op\}$\;
        }
    }
    $\text{acquire\_write\_locks}(write\_set)$\;
    $commit\_epoch \gets \text{get\_global\_epoch}()$\;
    \ForEach{$\langle k, v \rangle \in read\_set$}{
        \If{$v \ne \text{get\_current\_version}(k)$}{
            $\text{release\_write\_locks}()$; \Return{ABORT}\;
        }
    }
    \ForEach{$st \in read\_storages \cup scan\_storages$}{
        \ForEach{$\langle id, ep \rangle \in \text{get\_write\_preserves}(st)$}{
            \If{$ep \le commit\_epoch$}{
                $\text{release\_write\_locks}()$; \Return{ABORT}\;
            }
        }
    }
    \If{$\text{node\_verify}(node\_set) \ne \text{OK}$}{
        $\text{release\_write\_locks}()$; \Return{ABORT}\;
    }
    $\text{apply\_writes}(write\_set)$\;
    $\text{register\_reader\_epoch}(read\_set \cup scan\_storages, commit\_epoch)$\;
    $\text{release\_write\_locks}()$\;
    \Return{COMMIT}\;
}

\BlankLine

\SetKwBlock{FnRTX}{function \FExecRTX{$tx$}}{end}
\FnRTX{
    $snapshot\_epoch \gets \text{get\_safe\_snapshot\_epoch}()$\;
    \ForEach{$op \in tx$}{
        \eIf{$op.type = \text{READ}$}{
            $\text{read\_snapshot}(op.key, snapshot\_epoch)$\;
        }{
            $\text{scan\_snapshot}(op.range, snapshot\_epoch)$\;
        }
    }
    \Return{COMMIT}\;
}
\end{algorithm}

\begin{algorithm}[H]
\caption{Phantom Freedom Validation}
\DontPrintSemicolon
\SetKwBlock{FnVal}{function \FValidatePhantom{$write\_set, epoch$}}{end}
\FnVal{
    \ForEach{$op \in write\_set$}{
        \If{$op.type \in \{\text{INSERT, UPSERT, DELETE}\}$}{
            $readers \gets \text{get\_range\_readers}(op.key, epoch)$\;
            \If{$readers \ne \emptyset$}{ \Return{FALSE} }
        }
    }
    \Return{TRUE}\;
}
\end{algorithm}
