# Supplementary material for: Shirakami: A Hybrid Concurrency Control Protocol for Tsurugi Relational Database System
Source: arXiv:2303.18142 source file (2026-07-02)
Supplement: Supplementary file 2 [file appendix.tex]

\section{Tsurugi Access Layers}
Conventional commercial database systems, including open-source software, have a monolithic structure that assumes use only from the SQL layer. This is a remnant of the era when CPU, memory, and disk resources were scarce, and in order to use up resources efficiently, it was necessary to reduce unnecessary overhead and adopt the most efficient architecture possible. 
As a result, the key-value store (KVS) was forced to add transactional functions to KVS, or conversely, KVS interfaces were retrofitted to SQL-based relational database systems. We propose a so-called NewSQL component-based architecture.

Tsurugi has three access layers. They are the SQL layer, the user-defined function layer, and the key-value store layer. 

\subsection{SQL Access Layer}
This layer must be able to interoperate with PostgreSQL-compatible applications. There are already many relational database systems assets. It is necessary to be able to reuse them as much as possible. Many S/W and cloud services used by users can be connected if they are PostgreSQL-compatible. Therefore, the PostgreSQL-compatible interface was made accessible to Tsurugi's table with PostgreSQL's foreign data wrapper (FDW), which is useful.

In addition, it is necessary to be able to process in SQL, since access to a relational database is usually done through SQL, so it is necessary to have an SQL processor ready. 
SQL includes sub-queries, which requires non-deterministic reads and writes. Therefore the deterministic method does not help us.
In addition, the idea that, this should be solved by deterministic, is not valid for long transactions.

\subsection{User Defined Function Access Layer}
Some users require a user-defined function (UDF) to manipulate databases.
This is an interface for data batch registration or extraction M2M that uses simple data registration/extraction CVS, etc., and performs complex data registration/extraction (ETL processing).
A query is a process to narrow down data. It is required to be able to describe procedural processing, not declarative like SQL. In particular, batch processing, which requires long process descriptions, cannot be written in SQL.

\subsection{Key Value Store Access Layer}
This layer accesses the DB directly in a key-value style without the overhead of an SQL or UDF layer.
It has interfaces such as put, get, and scan. It also provides an interface that allows predicate processing.

\section{Telecommunication Billing Benchmark}
\begin{figure*}[tb]
 \centering
 \includegraphics[scale=1.0]{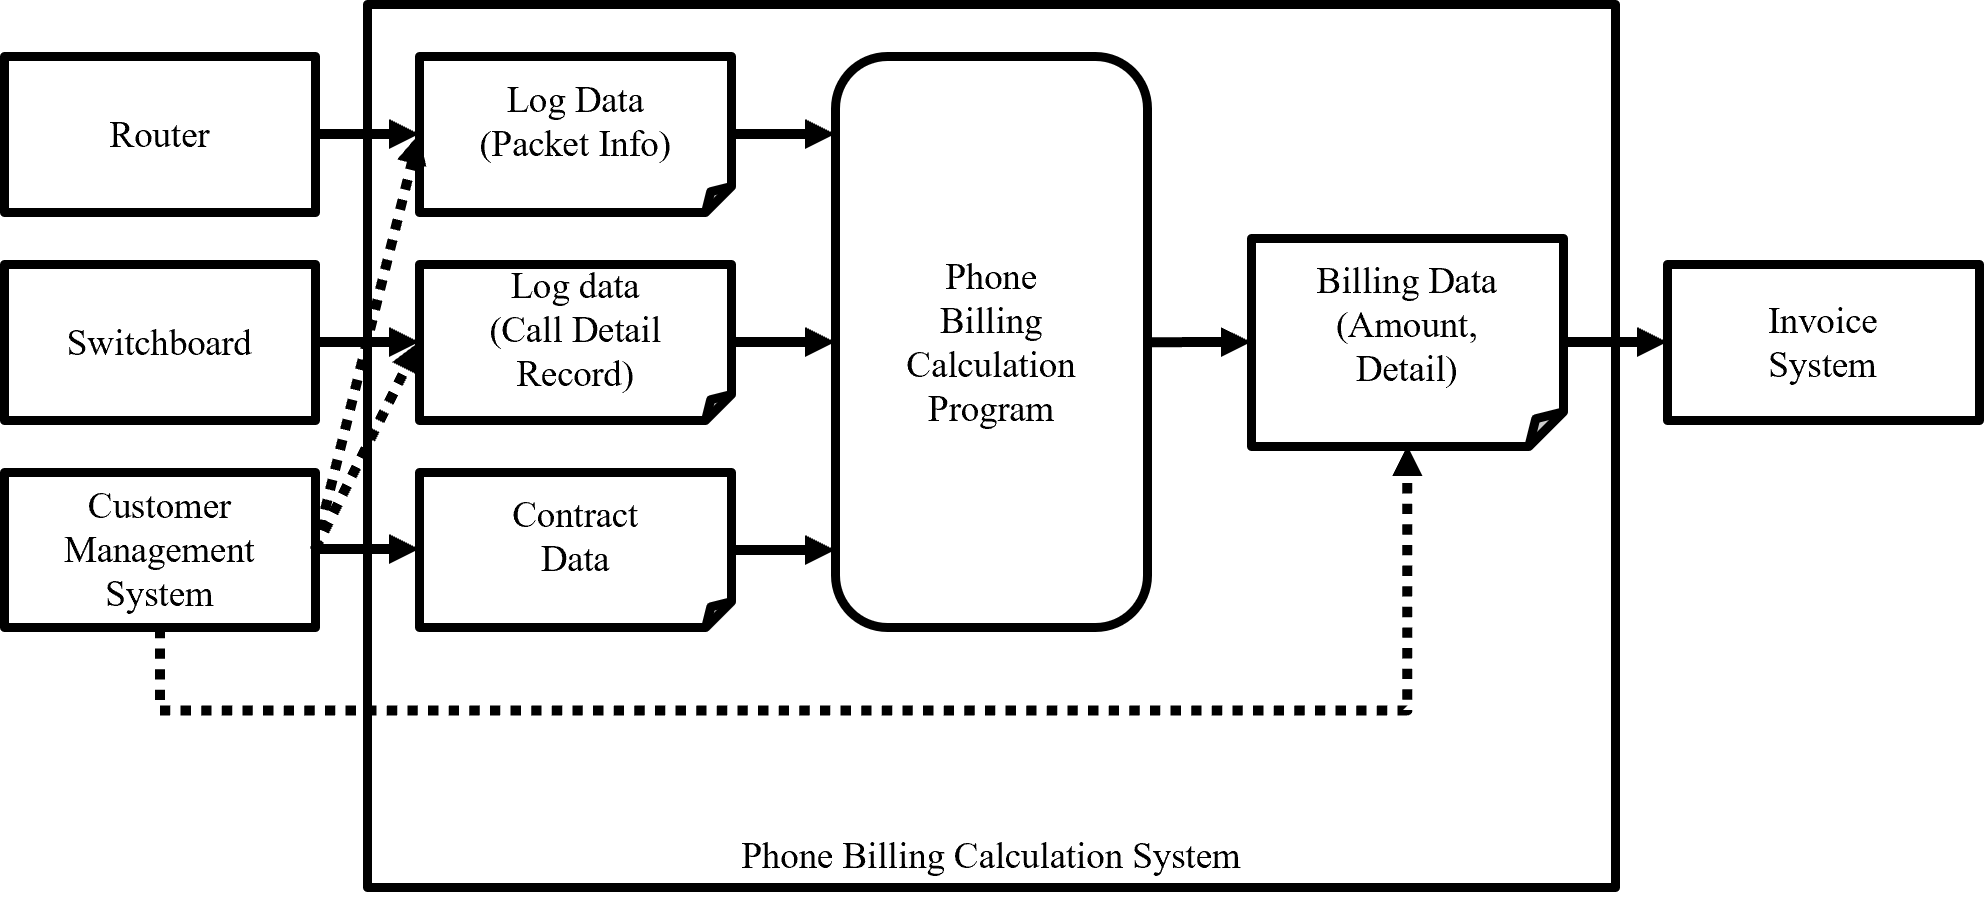}
 \caption{Billing System}
 \label{fig:Billing System}
\end{figure*}

We describe a telecommunication-based billing processing benchmark. This benchmark is a billing system for a fictitious telecommunication company described in Section \ref{sec:Shirakami-LTX}. The architecture is illustrated in Figure \ref{fig:Billing System}.

The telecommunication company provides cellular and fixed-line telephone service and Internet access service.

This system accumulates log information from routers, switching equipment, etc. This system is linked to a customer management system and maintains contract information. The system performs rate calculations in batch processing by date and time and links the rate calculation results to the customer management system and billing system.
The customer management system refers to the rate calculation results when responding to user inquiries. The billing system retrieves data necessary for billing processing from the rate calculation results and processes the billing.

The assumed work outline is to collect and store log data generated by the router and switching equipment in real-time. The system will also be linked to the customer management system. Among the customer data maintained by the customer management system, a copy of the data in the customer management system is maintained for the contract information necessary for rate calculations, and additions and updates to the data in the customer management system are reflected as appropriate.
The system also handles exceptional operations. For this purpose, the log data and the results of rate calculations are referenced and updated upon request from the customer management system.
Also, it performs rate calculations. The batch is executed on a daily basis to calculate rates for the current month and the previous month. The data for the current month is updated each time as historical data increases. Data for the previous month is calculated until the closing date and is no longer available for calculation after the closing date.

\subsection{Billing Calculation}
The call charge calculation process is as follows. In some cases, it is possible to determine from the call history whether the caller or the receiver will be billed for the call, and in other cases, it is not possible to know without matching the call history with the contract information. In some cases, no call charges are incurred when certain conditions are met. For each contract that calculates calling charges for each call based on the contract and records the calling charges for each call history, the calling history and calling charges to be calculated are picked up and totaled using the calculation method according to the contract, and the billing amount and billing details are prepared.

The packet rate calculation process is as follows. The packet information, IP information (information linking IP and contract), and contract information are matched to determine the contract to be billed. For each contract, packets that are subject to charge calculation are picked up, and the packets are totaled using a calculation method according to the contract, and the billing amount and billing details are created.
The system must be linked with the billing system, and the results of fee calculations are forwarded to the billing system based on requests from the billing system.

\subsection{Processed Data Size}
The approximate size of data to be stored and processed is as follows. First, contract information is about 5 million cases or 5 GB. Then, the log data of the switching system is described.
The information recorded in the log is call history, which includes the caller's phone number, received different phone number, call start time, call duration, etc. The size of one history is about 100 bytes. 10 million records are generated per day, and one year's worth of history must be maintained.

Router log data is also required. The information recorded in this log is packet information, including SRC IP, DST IP, port, timestamp, packet size, etc. Each history is about 30 bytes, and 100 billion records are generated per day. Therefore, 3 TByte/day, or 600 TB if two months' worth of history is stored.

Rate calculation results are also required. The number of active subscriptions in the subscription information is the result of the rate calculation. 5 KB per subscription. 250 GB for 2 months of calculation results.

\section{Bill of Materials Benchmark}
We use a food manufacturing company that produces bread nationwide as our reference when designing the BoMB workload. In the target food manufacturing industry, the supply chain can be disrupted by various reasons such as climate change, and the prices
of raw materials often change as well. Therefore, it is necessary to accurately gauge manufacturing costs and schedule an optimal production plan and supply chain. In order to reflect such needs, the BoMB workload is configured assuming a system capable of on-demand inventory control, cost control, and production planning.

We assume that the target system consists of a manufacturing resource planning (MRP) system that manages products and resources needed for manufacturing and a perpetual inventory management system that continuously manages the inventory. The MRP consists of cost management, budgeting, demand planning, and supply chain management (SCM) modules, and each module accesses one database. Cost management generates the most complicated workload among these modules due to the
long-running update transactions. Thus, for BoMB, we focus on emulating the workload of the cost management module.

The BoMB workload has six transactions that are directly related to product costing and its input/output: L1 and S1, $\cdots$, and 5 transactions.
L and S stand for long and short respectively. All of these transactions generally occur in manufacturing industries and can be widely applied other than in bakeries. The details of this benchmark are found in \cite{Nemoto22oze}.
